# Supplementary material for: Computed tomography of propagating microwave photons
Source: arXiv:2506.20318 ancillary file (2025-07-02)
Supplement: Supplementary file 1 [file BoloCT_sup.pdf]

# Supplemental Information for
# "Computed tomography of propagating microwave photons"

(Dated: July 2, 2025)

## CONTENTS


Supplementary Note 1. Gaussian-state generator. 1

Supplementary Note 2. Two-photon interference 2

Supplementary Note 3. Bolometry characterization 2

Supplementary Note 4. Computed tomography 3

Supplementary Note 5. Compressed sensing 4

Supplementary Note 6. Ultra-sparse sampling 5

## Supplementary Note 1. GAUSSIAN-STATE GENERATOR.

A Gaussian state of a bosonic field with annihilation operator $\hat{a}$ is defined as a squeezed and displaced thermal state given by

$$\hat{\rho}_{\mathrm{G}} = \hat{D}(\alpha)\hat{S}\left(\zeta\right)\hat{\rho}_T\hat{S}^{\dagger}\left(\zeta\right)\hat{D}^{\dagger}(\alpha), \tag{S1}$$

where $\hat{\rho}_T$ is a thermal state with mean photon number $\bar{n}_T$, and $\hat{S}(\zeta) = \exp\left(\zeta^*\hat{a}^2/2 - \zeta\hat{a}^{\dagger 2}/2\right)$ and $\hat{D}(\alpha) = \exp\left(\alpha\hat{a}^{\dagger} - \alpha^*\hat{a}\right)$ are the squeezing and displacement operators, respectively. In superconducting quantum circuits, thermal photons can be precisely generated by a blackbody radiator [35]. The squeezing operation can implemented using Josephson parametric amplifiers (JPAs) [7, 8, 46, 47], Josephson parametric converters (JPCs) [48–50], and Josephson traveling-wave parametric amplifiers (TWPAs) [36–38]. The displacement operation can be achieved by using a directional coupler [10].

Our experimental setup, shown in Extended Data Figs. 1 and 2, combines a blackbody radiator, a TWPA, and a directional coupler to generate arbitrary Gaussian states over a broad bandwidth. The optimal output frequency of the generator is between 4.5 and 6.5 GHz, mainly limited by the frequency doubler and filters in the squeezing line. However, we operate the generator at 8.43 GHz for bolometry because the superconductor–normal-metal–superconductor (SNS) bolometer has an on-chip coplanar waveguide filter at $f_0 = 8.43$ GHz with a FWHM = 133 MHz bandwidth. For the displacement and homodyne fields at this frequency, we observe an approximately 30 dB of added attenuation in the room-temperature setup. The estimated total attenuation of the displacement line is 100 dB (to the directional coupler input), and that of the homodyne line is 115 dB (to the beam splitter input). The homodyne line attenuation is fine-tuned during the characterization. For the double-frequency squeezing field at 16.86 GHz, we estimate a total attenuation of 115 dB from the source to the TWPA input. Here, the room-temperature setup contributes to an approximately 55 dB attenuation, which is confirmed by generating a 8.43 GHz signal at the source while measuring the power at 16.86 GHz.

One practical challenge in the current setup is the observed leakage at 8.43 GHz from the frequency doubler. It causes an undesired displacement of the Gaussian state before squeezing. Our solution is to actively compensate it by applying an additional displacement field. With a $-103$ dBm squeezing power (estimated at the TWPA input), we sweep the power and phase of the additional field and measure the oscillation of the thermometry lineshape with respect to the projection angle, $\phi$. Supplementary Figure 1A presents the oscillation magnitude as a function of the displacement power and phase. We fit the oscillation magnitude as a two-dimensional polynomial function of the control parameters, as shown in Supplementary Fig. 1B. The optimal parameters of the compensation field is located at the fitted minimum, which is $-102.3$ dBm at 170°, see Supplementary Fig. 1C.

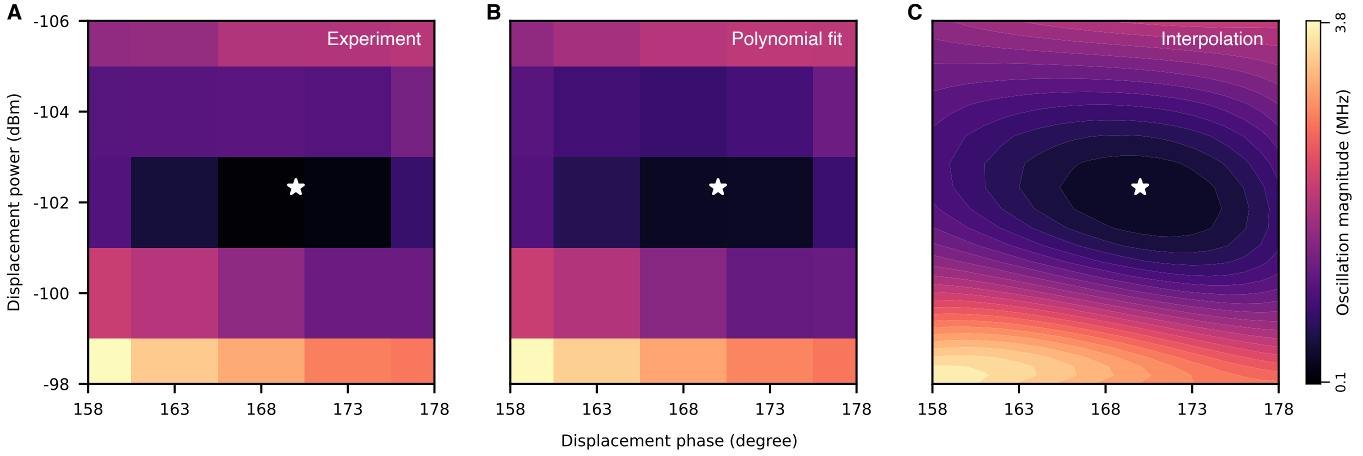


**Supplementary Fig. 1: Characterization of displacement.** **A** Measured oscillation magnitude of the thermometer resonance frequency as a function of displacement power (estimated at the directional coupler input) and phase. **B** Polynomial fit of the oscillation magnitude in A with up to 3 orders in both of the displacement power and phase. **C** Interpolation of B with refined power and phase axes, from which we locate the optimal compensation field at the star marker.

## Supplementary Note 2. TWO-PHOTON INTERFERENCE

We define the following input-output relation of a 90° hybrid

$$\begin{bmatrix}\hat{c}\\ \hat{d}\end{bmatrix} = \begin{bmatrix}\sqrt{\Gamma} & \mathrm{i}\sqrt{1-\Gamma}\\ \mathrm{i}\sqrt{1-\Gamma} & \sqrt{\Gamma}\end{bmatrix}\begin{bmatrix}\hat{a}\\ \hat{b}\end{bmatrix}, \tag{S2}$$

where $\Gamma$ is the transmissivity, $\hat{a}$, $\hat{b}$, $\hat{c}$, and $\hat{d}$ are the field operators at the four different ports that are often denoted as input, isolated, and outputs 1 and 2. Specific to the field at output 1, which is the input field of the SNS bolometer, we have

$$\langle\hat{n}_c\rangle = \Gamma\langle\hat{n}_a\rangle + (1-\Gamma)\langle\hat{n}_b\rangle + \mathrm{i}\sqrt{\Gamma(1-\Gamma)}\left(\langle\hat{a}^\dagger\rangle\langle\hat{b}\rangle - \langle\hat{a}\rangle\langle\hat{b}^\dagger\rangle\right), \tag{S3}$$

where $\hat{n}_y = \hat{y}^\dagger\hat{y}$ is the photon number operator for the field $\hat{y}$. We assume that the homodyne field, $\hat{b}$, is prepared in a coherent state $|\beta\rangle$ with $\beta = |\beta|\mathrm{e}^{\mathrm{i}\phi}$, so that the above equation can be simplified as

$$\langle\hat{n}_c\rangle = \Gamma\langle\hat{n}_a\rangle + (1-\Gamma)|\beta|^2 + \sqrt{2\Gamma(1-\Gamma)}|\beta|\langle\hat{X}_{\phi+90}\rangle, \tag{S4}$$

Here, $\hat{X}_\phi = (\hat{a}^\dagger\mathrm{e}^{\mathrm{i}\phi} + \hat{a}\mathrm{e}^{-\mathrm{i}\phi})/\sqrt{2}$ is a quadrature operator of the input field $\hat{a}$.

We define the photon number variance of field $\hat{y}$ as $\langle(\Delta\hat{n}_y)^2\rangle = \langle\hat{n}_y^2\rangle - \langle\hat{n}_y\rangle^2$. Considering the field $\hat{c}$ of interest, we have

$$\begin{aligned}\langle(\Delta\hat{n}_c)^2\rangle = {}& (1-\Gamma)|\beta|^2\left[(1-\Gamma) + 2\Gamma\langle(\Delta\hat{X}_{\phi+90})^2\rangle\right] + \Gamma^2\langle(\Delta\hat{n}_a)^2\rangle + \Gamma(1-\Gamma)\langle\hat{n}_a\rangle\\ &+ \sqrt{\Gamma(1-\Gamma)}|\beta|\left[\mathrm{i}\Gamma\left(2\langle\hat{a}^\dagger\hat{a}^\dagger\hat{a}\rangle\mathrm{e}^{\mathrm{i}\phi} - 2\langle\hat{a}^\dagger\hat{a}\hat{a}\rangle\mathrm{e}^{-\mathrm{i}\phi}\right) + \sqrt{2}\left(1-2\Gamma\langle\hat{n}_a\rangle\right)\langle\hat{X}_{\phi+90}\rangle\right],\end{aligned} \tag{S5}$$

where $\langle(\Delta\hat{X}_\phi)^2\rangle = \left[\langle(\Delta\hat{a}^\dagger)^2\rangle\mathrm{e}^{\mathrm{i}2\phi} + \langle(\Delta\hat{a})^2\rangle\mathrm{e}^{-i2\phi} + 2\left(\langle\hat{n}_a\rangle - \langle\hat{a}^\dagger\rangle\langle\hat{a}\rangle\right) - 1\right]/2$.

For a thermal input state with mean photon number $\bar{n}_T$, we can simplify the above equations as

$$\langle\hat{n}_c\rangle = \Gamma\bar{n}_T + (1-\Gamma)|\beta|^2, \tag{S6}$$

$$\langle(\Delta\hat{n}_c)^2\rangle = \Gamma^2\bar{n}_T^2 + \Gamma\bar{n}_T\left[2(1-\Gamma)|\beta|^2 + 1\right] + (1-\Gamma)|\beta|^2. \tag{S7}$$

For a coherent input state with displacement $\alpha = |\alpha|\mathrm{e}^{\mathrm{i}\theta}$, we have

$$\langle\hat{n}_c\rangle = \Gamma|\alpha|^2 + (1-\Gamma)|\beta|^2 - 2\sqrt{\Gamma(1-\Gamma)}|\alpha||\beta|\sin(\phi-\theta), \tag{S8}$$

$$\langle(\Delta\hat{n}_c)^2\rangle = \Gamma|\alpha|^2 + (1-\Gamma)|\beta|^2 - 2\sqrt{\Gamma(1-\Gamma)}|\alpha||\beta|\sin(\phi-\theta). \tag{S9}$$

In general, we have the following relations for large $|\beta|^2$, which are Eqs. (1) and (2) of the main text

$$\langle\hat{n}_c\rangle = \Gamma\langle\hat{n}_a\rangle + (1-\Gamma)|\beta|^2 + \sqrt{2\Gamma(1-\Gamma)|\beta|^2}\langle\hat{X}_\phi\rangle, \tag{S10}$$

$$\langle(\Delta\hat{n}_c)^2\rangle \approx (1-\Gamma)|\beta|^2\left[(1-\Gamma) + 2\Gamma\langle(\Delta\hat{X}_\phi)^2\rangle\right]. \tag{S11}$$

Note that Eq. (S11) is obtained by keeping only the leading order term of $|\beta|^2$ in Eq. (S5).

## Supplementary Note 3. BOLOMETRY CHARACTERIZATION

The characterization of the measurement setup is based on Eqs. (S6) and (S7) for thermal input states. When applying radiation to the bolometer, we measure its response by sweeping a weak thermometry field at sub-gigahertz frequencies. On average, the mean resonance frequency, $\mu$, of the reflection spectrum is determined by the mean input photon number, $\langle\hat{n}_c\rangle$, and the Gaussian broadening, $\sigma^2$, is determined by the photon number variance, $\langle(\Delta\hat{n}_c)^2\rangle$ [30]. Thus, a contour of $\mu$ or $\sigma^2$ indicates a constant photon number $\langle\hat{n}_c\rangle$ or variance $\langle(\Delta\hat{n}_c)^2\rangle$, respectively. Without loss of generality, we define $\langle\hat{n}_c\rangle = f(\mu)$ and $\langle(\Delta\hat{n}_c)^2\rangle = g(\sigma^2)$, where $f(\cdot)$ and $g(\cdot)$ are arbitrary functions to be characterized.

During the characterization, we generate thermal states with different populations, $\bar{n}_T$. The homodyne photon number is calculated as $|\beta|^2 = \eta_1 P_\mathrm{h}/(\mathrm{FWHM}hf_0)$, where $P_\mathrm{h}$ is the estimated homodyne power at the beam splitter

input with $\eta_1$ being a possible correction. In addition, $f_0 = 8.43\,\mathrm{GHz}$ and $\mathrm{FWHM} = 133\,\mathrm{MHz}$ are the central frequency and bandwidth of an on-chip filter between the beam splitter and the bolometer, and $h$ is Planck's constant. At each contour of $\mu$ and $\sigma^2$, we rewrite Eqs. (S6) and (S7) as

$$\frac{f(\mu)}{(1-\Gamma)\eta_1} = \frac{\Gamma\bar{n}_T}{(1-\Gamma)\eta_1} + \frac{P_\mathrm{h}}{\mathrm{FWHM}hf_0}, \tag{S12}$$

$$\frac{g(\sigma^2)}{\Gamma} = \Gamma\bar{n}_T^2 + \bar{n}_T + (2\Gamma\bar{n}_T + 1)\frac{(1-\Gamma)\eta_1}{\Gamma}\frac{P_\mathrm{h}}{\mathrm{FWHM}hf_0}. \tag{S13}$$

We further consider an $\eta_0 = -6.5\,\mathrm{dB}$ correction of the thermal photon number, such that $\bar{n}_T = \eta_0/\left\{\exp\left[hf_0/(k_\mathrm{B}T)\right] - 1\right\}$ with $k_\mathrm{B}$ being the Boltzmann constant. This choice of $\eta_0$ is the sum of the insertion loss between the blackbody radiator and the beam splitter input, which consists of one DC block (Fairview MW, SD3258, 0.75 dB), one filter (Mini-circuits, VHF-3800+, 0.7 dB), three circulators (QUINSTAR, QCI-075900X000, 1.28 dB; LNF, ISC412A, $2 \times 0.2$ dB), two directional couplers (KRYTAR, 12040, $2 \times 0.9$ dB), and the two switches (Radiall, R573432600, 0.4 dB; Radiall, R570433000, 0.25 dB). The characterization of a TWPA similar to that used in our experiments indicates a frequency-dependent insertion loss between 0.5 and 2 dB [36]. Here, we choose 0.92 dB insertion loss of the TWPA to obtain $\eta_0 = -6.5\,\mathrm{dB}$. A $\pm 0.5\,\mathrm{dB}$ change of $\eta_0$ only leads to a marginal change of the characterization result. We note that $\eta_0$ is only used for characterization purposes, but not for quadrature bolometry and Wigner function computed tomography (CT).

Fitting the linear equation, i.e., Eq. (S12), we obtain the two parameters $\Gamma\eta_0/[(1-\Gamma)\eta_1]$ and $f(\mu)/[(1-\Gamma)\eta_1]$. Consequently, there are only two parameters left, $\Gamma\eta_0$ and $g(\sigma^2)/(\Gamma\eta_1)$, which can be fitted via the quadratic equation, i.e., Eq. (S13). These fitted results can deterministically define the four parameters $f(\mu)$, $g(\sigma^2)$, $\Gamma$, and $\eta_1$ at each fixed $\mu$ and $\sigma^2$. In the end, we obtain $\Gamma = 0.49$ and $\eta_1 = -3.4\,\mathrm{dB}$. The characterized transmissivity of the 90° hybrid, $\Gamma$, is in quantitative agreement with the datasheet value (MCLI, HB-63).

## Supplementary Note 4. COMPUTED TOMOGRAPHY

The beam splitter interaction enables quadrature measurement with a power detector. In our experiment, we first read out $\langle\hat{n}_c\rangle$ and $\langle(\Delta\hat{n}_c)^2\rangle$ by fitting the resonance frequency, $\mu$, and Gaussian broadening, $\sigma^2$, with the Voigt profile. The mean and variance of the quadrature operator, $\hat{X}_\phi$, are obtained thereafter from Eqs. (S10) and (S11). We generate the marginal distributions of the input state at different projection angles by assuming a Gaussian distribution, i.e.,

$$h_\phi(x_\phi) = \frac{1}{\sqrt{2\pi\langle(\Delta\hat{X}_\phi)^2\rangle}}\exp\left[-\frac{\left(x_\phi - \langle\hat{X}_\phi\rangle\right)^2}{2\langle(\Delta\hat{X}_\phi)^2\rangle}\right]. \tag{S14}$$

Here, $x_\phi$ represents one sampling of the quadrature operator $\hat{X}_\phi$. On the other hand, $h_\phi(x_\phi)$ can be calculated from the Wigner function by an integration over the conjugate variable, $p_\phi$, i.e., [31]

$$h_\phi\left(x_\phi\right) = \int \mathrm{d}p_\phi\, W\left(x_\phi\cos\phi - p_\phi\sin\phi, x_\phi\sin\phi + p_\phi\cos\phi\right). \tag{S15}$$

By definition, $p$ is the eigenvalue of the quadrature operator $\hat{X}_{\phi+90}$, where $\left[\hat{X}_\phi, \hat{X}_{\phi+90}\right] = \mathrm{i}$ with $\hbar = 1$. This formula is known as the Radon transform by treating the Wigner function, $W(x,p)$, as a two-dimensional gray-scale image.

For the first-order term, $\langle\hat{X}_\phi\rangle$, we note that it must be a trigonometric function of $\phi$ with zero mean and 360° periodicity. Subtracting the measured $\langle\hat{n}_c\rangle$ with its mean value, we obtain

$$\langle\hat{X}_\phi\rangle = -\frac{\langle\hat{n}_c\rangle - \overline{\langle\hat{n}_c\rangle}}{2\sqrt{\Gamma(1-\Gamma)|\beta|^2}}. \tag{S16}$$

Here, the average $\overline{x}$ is taken over $\phi$. On the other hand, the second-order term, $\langle(\Delta\hat{X}_\phi)^2\rangle$, must also have an 180° periodicity but with a possibly finite mean value. We extract $\langle(\Delta\hat{X}_\phi)^2\rangle$ by inserting the characterization result of $\Gamma$ and $|\beta|^2$ into Eq. (S11), i.e.,

$$\langle(\Delta\hat{X}_\phi)^2\rangle \approx \frac{\langle(\Delta\hat{n}_c)^2\rangle}{4\Gamma(1-\Gamma)|\beta|^2} - \frac{1-\Gamma}{4\Gamma}. \tag{S17}$$

We note that there is no fitting parameter in extracting $\langle\hat{X}_\phi\rangle$ and $\langle(\Delta\hat{X}_\phi)^2\rangle$, nor assumption of the input state. In later experiments of Wigner function CT, we use the extracted values of $\langle\hat{X}_\phi\rangle$ and $\langle(\Delta\hat{X}_\phi)^2\rangle$ to generate Gaussian distributions as projected histograms of the Wigner function. The generated Gaussian distributions at different $\phi$ are independent measurement results from each other, which not necessarily result in a Gaussian form of the reconstructed Wigner function.

With the projected histograms at different angles, reconstruction of the Wigner function can be achieved by following the same methodology of CT in medical science [33]. We first apply the Fourier transform on both sides of Eq. (S15) with respect to the variable $x_\phi$, and obtain

$$\tilde{h}_\phi\left(\omega_\phi\right)=\int \mathrm{d}x\int \mathrm{d}p\, W\left(x,p\right)\exp\left[-\mathrm{i}2\pi\omega_\phi\left(x\cos\phi+p\sin\phi\right)\right]=\tilde{W}(\Omega_x,\Omega_p), \tag{S18}$$

where $\tilde{W}(\Omega_x,\Omega_p)$ is the Fourier transform of $W(x,p)$ with $\Omega_x=\omega_\phi\cos\phi$ and $\Omega_p=\omega_\phi\sin\phi$. This result is called the central slice theorem in CT [33], which indicates

$$\begin{aligned}W\left(x,p\right)&=\int \mathrm{d}\Omega_x\int \mathrm{d}\Omega_p\tilde{W}(\Omega_x,\Omega_p)\exp\left[\mathrm{i}2\pi\left(x\Omega_x+p\Omega_p\right)\right]\\&=\frac{1}{2\pi}\int_0^\pi \mathrm{d}\phi\left[\frac{1}{\pi x_\phi}*\frac{\partial h_\phi(x_\phi)}{\partial x_\phi}\right]\Big|_{x_\phi=x\cos\phi+p\sin\phi}\end{aligned} \tag{S19}$$

Here, the convolution with $1/(\pi x_\phi)$ is called the Hilbert transform.

## Supplementary Note 5. COMPRESSED SENSING

We discretize the Wigner function into $M\times M$ pixels with $M$ being an odd number, and define the index $(0,0)$ at the center. This image can be stretched into a one-dimensional vector $[W_1,\cdots,W_{M^2}]^\mathrm{T}$, where the elements are the Wigner function evaluated at the indexes $[(-N,-N),(-N,N+1),\cdots,(N,N)]^\mathrm{T}$ up to a scaling factor of the integration area. To describe the projective measurement at angle $\phi$, we fix the image but rotate the axis by $-\phi$ about the origin. Thus, the pixel $(n_x,n_y)$ is moved to the new position

$$\begin{bmatrix}x'\\y'\end{bmatrix}=\begin{bmatrix}\cos(\phi)&\sin(\phi)\\-\sin(\phi)&\cos(\phi)\end{bmatrix}\begin{bmatrix}n_x\\n_y\end{bmatrix}. \tag{S20}$$

We refer to this new image as $W'(x',y')$. Because $x'$ and $y'$ are not necessarily integers, we resample the image at the integer values of $x'$. Using linear interpolation, if $x'$ is between two integers $n'_x$ and $(n'_x+1)$, we split it into two values, $(1-\kappa)W(n'_x,y')$ and $\kappa W(n'_x+1,y')$, and assign them to the indexes $(n'_x,y')$ and $(n'_x+1,y')$, respectively. Here, $\kappa=x'-n'_x$ is a normalization factor that keeps the sum over the indexes unchanged. Note that it is not necessary to convert $y'$ to an integer because we sum over this axis to get the result of projective measurement. Consequently, the quadrature bolometry at angle $\phi$ can be described as

$$\begin{bmatrix}P_1\\P_2\\\vdots\\P_{M'}\\P_{M'+1}\end{bmatrix}=\begin{bmatrix}(1-\kappa_{1,1})&\cdots&(1-\kappa_{1,M^2})&0&\cdots&0\\(1-\kappa_{2,1})&\cdots&(1-\kappa_{2,M^2})&\kappa_{1,1}&\cdots&\kappa_{1,M^2}\\\vdots&&\vdots&\vdots&&\vdots\\(1-\kappa_{M',1})&\cdots&(1-\kappa_{M',M^2})&\kappa_{M'-1,1}&\cdots&\kappa_{M'-1,M^2}\\0&\cdots&0&\kappa_{M',1}&\cdots&\kappa_{M',M^2}\end{bmatrix}\begin{bmatrix}W_1\\\vdots\\W_{M^2}\\W_1\\\vdots\\W_{M^2}\end{bmatrix}, \tag{S21}$$

where the vector $[P_1,\cdots,P_{M'+1}]^\mathrm{T}$ is the projected histogram, and we choose $M'=2\times\mathrm{ceil}[(M-1)/\sqrt{2}]$ to cover the full range of the argument for the projected histogram.

For simplicity, we write the above equation in a compact form $\mathbf{P}_\phi=\mathbb{A}_\phi\mathbf{W}$, where the subscript $\phi$ explicitly defines the projection angle. We can stack the measurement results of $N$ projection angles, $\phi_1,\phi_2,\cdots,\phi_N$, as

$$\begin{bmatrix}\mathbf{P}_{\phi_1}\\\mathbf{P}_{\phi_2}\\\vdots\\\mathbf{P}_{\phi_N}\end{bmatrix}=\begin{bmatrix}\mathbb{A}_{\phi_1}\\\mathbb{A}_{\phi_2}\\\vdots\\\mathbb{A}_{\phi_N}\end{bmatrix}\mathbf{W}. \tag{S22}$$

This equation reformulates the CT problem as a set of linear equations, $\mathbf{P}_N = \mathbb{A}_N\mathbf{W}$ where $\mathbf{P}_N = [\mathbf{P}_{\phi_1}, \mathbf{P}_{\phi_2}, \cdots, \mathbf{P}_{\phi_N}]^{\mathrm{T}}$ and $\mathbb{A}_N = [\mathbb{A}_{\phi_1}, \mathbb{A}_{\phi_2}, \cdots, \mathbb{A}_{\phi_N}]^{\mathrm{T}}$. Note that the matrix, $\mathbb{A}_N$, has a dimension of $N(M'+1) \times M^2$, such that the system is under-defined when $N < M^2/(M'+1)$ and over-defined otherwise. In principle, it is possible to find a unique solution of $\mathbf{W}$ when $N \geq M^2/(M'+1)$, which is indicated by the Shannon–Nyquist sampling theorem.

One may bypass the sampling theorem by using the advanced signal processing method, known as compressed sensing (CS) [40, 41]. This method looks for a solution with the highest sparsity in a certain basis. A successful application of CS has two requirements: (i) $\mathbf{W}$ can be sparsely represented in the chosen basis, i.e., $\mathbf{W} = \mathbb{B}\mathbf{W}'$ where $\mathbb{B}$ is the sparse-representing matrix and $\mathbf{W}'$ is a sparse vector. (ii) The sensing matrix, $\mathbb{A}_N\mathbb{B}$, should fulfill the so-called restricted isometry property (RIP). Another expression of RIP is that $\mathbb{A}_N$ and $\mathbb{B}$ are incoherent from each other in the sense that each column vector of $\mathbb{A}_N$ ($\mathbb{B}$) cannot be sparsely represented by those of $\mathbb{B}$ ($\mathbb{A}_N$). An illustrative example is an identity matrix as $\mathbb{A}_N$ and a discrete Fourier transform (DCT) matrix as $\mathbb{B}$, where the uncertainty principle inherent to the Fourier transform pair guarantees the incoherence between them. In common practices of image processing, the RIP is often loosely assumed.

In our example, we choose $N$ evenly spaced projection angles for CS. We do not observe a clear advantage when choosing random projection angles. We use two sparse-representing matrices, $\mathbb{B}$, for demonstration purpose, which correspond to the DCT and the Daubechies wavelet transform, respectively. In the optimization approach, we use the Lasso optimizer from the scikit-learn package to minimize the $\ell^1$-norm of $\mathbf{W}'$. In the iterative approach, we first use the Hilbert transform to obtain $\mathbf{W}$. Then, we look for the largest component in the sparse-representing basis and subtract it from $\mathbf{W}'$ in each iteration. We repeat this process until the largest component of $\mathbf{W}'$ is less than 5 times of the standard deviation. This procedure is sometimes referred to as the iterative method with soft thresholding.

## Supplementary Note 6. ULTRA-SPARSE SAMPLING

Considering a Gaussian state of the input field, $\hat{a}$, we have

$$\langle\hat{a}\rangle = \alpha,\ \langle\hat{a}^2\rangle = -\left(\bar{n}_T + \frac{1}{2}\right)\sinh(2r)\mathrm{e}^{\mathrm{i}2\varphi} + \alpha^2,\ \langle\hat{a}^\dagger\hat{a}\rangle = \left(\bar{n}_T + \frac{1}{2}\right)\cosh(2r) + |\alpha|^2 - \frac{1}{2}, \tag{S23}$$

where $\bar{n}_T$ is the thermal photon number, $\zeta = r\mathrm{e}^{\mathrm{i}2\varphi}$ the squeezing parameter, and $\alpha = |\alpha|\mathrm{e}^{\mathrm{i}\theta}$ the displacement parameter. Correspondingly, we derive the following expressions of the quadrature mean and variance

$$\langle\hat{X}_{\phi+90}\rangle = -\sqrt{2}|\alpha|\sin(\phi-\theta), \tag{S24}$$

$$\langle(\Delta\hat{X}_{\phi+90})^2\rangle = \frac{2\bar{n}_T+1}{2}\left\{\sinh(2r)\cos[2(\phi-\varphi)] + \cosh(2r)\right\}. \tag{S25}$$

These results allow us to use trigonometric functions with periodicity 360° and 180°, respectively, to fit the measurement results and to determine the parameters $\bar{n}_T$, $\zeta$, and $\alpha$. From Eq. (S25), we observe that the maximum and minimum values of $\langle(\Delta\hat{X}_{\phi+90})^2\rangle$ can be written as

$$\langle(\Delta\hat{X})^2\rangle_{\max/\min} = (2\bar{n}_T+1)\mathrm{e}^{\pm 2r}/2. \tag{S26}$$

Thus, the thermal population and the squeezing parameter can be calculated as

$$\bar{n}_T = \frac{1}{2}\left(2\sqrt{\langle(\Delta\hat{X})^2\rangle_{\max}}\sqrt{\langle(\Delta\hat{X})^2\rangle_{\min}} - 1\right), \tag{S27}$$

$$r = \frac{1}{2}\ln\left(\sqrt{\langle(\Delta\hat{X})^2\rangle_{\max}}/\sqrt{\langle(\Delta\hat{X})^2\rangle_{\min}}\right). \tag{S28}$$

The squeezing level is defined as $S = 20r\,\lg(e)$.

The above result indicates that a general Gaussian state can be fully determined by three projective measurements, assuming that the measurements are free from noise. Considering the unavoidable noise in practice, we apply two methods to approach this limit: Linear least-squares regression (LLS) and neural network (NN). In LLS, we use Eqs. (S24) and (S25) to fit the experimental data measured at $\phi = 0°$, 60°, and 120° and obtain $\bar{n}_T$, $\zeta$, and $\alpha$. Alternatively, we train a three-layer NN with a linear input layer of 6 neurons, a sigmoid hidden layer of 128 neurons, and a linear output layer of 5 neurons. The input data are $\langle\hat{X}_{\phi+90}\rangle$ and $\langle(\Delta\hat{X}_{\phi+90})^2\rangle$ evaluated at $\phi = 0°$, 60°, and 120°, while the output data are the corresponding values of $\bar{n}_T$, $\mathrm{Re}(\zeta)$, $\mathrm{Im}(\zeta)$, $\mathrm{Re}(\alpha)$, and $\mathrm{Im}(\alpha)$. The training is

performed with the PyTorch package, where we use the Adam algorithm with a learning rate of $10^{-2}$. We generate 32768 training data according to Eqs. (S24) and (S25), and optimize the weights of the NN by 100 epochs with 256 batch size. In the end, we obtain a NN with a mean squared error (MSE) smaller than 0.001, which is used for Wigner function CT with ultra-sparse sampling.

---


[1] M. Hofheinz, H. Wang, M. Ansmann, R. C. Bialczak, E. Lucero, M. Neeley, A. D. O'Connell, D. Sank, J. Wenner, J. M. Martinis, and A. N. Cleland, Synthesizing arbitrary quantum states in a superconducting resonator, Nature **459**, 546 (2009).

[2] L. Sun, A. Petrenko, Z. Leghtas, B. Vlastakis, G. Kirchmair, K. M. Sliwa, A. Narla, M. Hatridge, S. Shankar, J. Blumoff, L. Frunzio, M. Mirrahimi, M. H. Devoret, and R. J. Schoelkopf, Tracking photon jumps with repeated quantum non-demolition parity measurements, Nature **511**, 444 (2014).

[3] G. Kirchmair, B. Vlastakis, Z. Leghtas, S. E. Nigg, H. Paik, E. Ginossar, M. Mirrahimi, L. Frunzio, S. M. Girvin, and R. J. Schoelkopf, Observation of quantum state collapse and revival due to the single-photon kerr effect, Nature **495**, 205 (2013).

[4] E. P. Menzel, F. Deppe, M. Mariantoni, M. A. Araque Caballero, A. Baust, T. Niemczyk, E. Hoffmann, A. Marx, E. Solano, and R. Gross, Dual-path state reconstruction scheme for propagating quantum microwaves and detector noise tomography, Phys. Rev. Lett. **105**, 100401 (2010).

[5] C. Eichler, D. Bozyigit, C. Lang, L. Steffen, J. Fink, and A. Wallraff, Experimental state tomography of itinerant single microwave photons, Phys. Rev. Lett. **106**, 220503 (2011).

[6] C. Eichler, D. Bozyigit, C. Lang, M. Baur, L. Steffen, J. M. Fink, S. Filipp, and A. Wallraff, Observation of two-mode squeezing in the microwave frequency domain, Phys. Rev. Lett. **107**, 113601 (2011).

[7] E. P. Menzel, R. Di Candia, F. Deppe, P. Eder, L. Zhong, M. Ihmig, M. Haeberlein, A. Baust, E. Hoffmann, D. Ballester, K. Inomata, T. Yamamoto, Y. Nakamura, E. Solano, A. Marx, and R. Gross, Path entanglement of continuous-variable quantum microwaves, Phys. Rev. Lett. **109**, 250502 (2012).

[8] L. Zhong, E. P. Menzel, R. Di Candia, P. Eder, M. Ihmig, A. Baust, M. Haeberlein, E. Hoffmann, K. Inomata, T. Yamamoto, Y. Nakamura, E. Solano, F. Deppe, A. Marx, and R. Gross, Squeezing with a flux-driven josephson parametric amplifier, New J. Phys. **15**, 125013 (2013).

[9] E. Flurin, N. Roch, J. D. Pillet, F. Mallet, and B. Huard, Superconducting quantum node for entanglement and storage of microwave radiation, Phys. Rev. Lett. **114**, 090503 (2015).

[10] K. G. Fedorov, L. Zhong, S. Pogorzalek, P. Eder, M. Fischer, J. Goetz, E. Xie, F. Wulschner, K. Inomata, T. Yamamoto, Y. Nakamura, R. Di Candia, U. Las Heras, M. Sanz, E. Solano, E. P. Menzel, F. Deppe, A. Marx, and R. Gross, Displacement of propagating squeezed microwave states, Phys. Rev. Lett. **117**, 020502 (2016).

[11] Q.-M. Chen, M. Fischer, Y. Nojiri, M. Renger, E. Xie, M. Partanen, S. Pogorzalek, K. G. Fedorov, A. Marx, F. Deppe, and R. Gross, Quantum behavior of the duffing oscillator at the dissipative phase transition, Nat. Commun. **14**, 2896 (2023).

[12] C. Eichler, D. Bozyigit, and A. Wallraff, Characterizing quantum microwave radiation and its entanglement with superconducting qubits using linear detectors, Phys. Rev. A **86**, 032106 (2012).

[13] Y.-F. Chen, D. Hover, S. Sendelbach, L. Maurer, S. T. Merkel, E. J. Pritchett, F. K. Wilhelm, and R. McDermott, Microwave photon counter based on josephson junctions, Phys. Rev. Lett. **107**, 217401 (2011).

[14] K. Inomata, Z. Lin, K. Koshino, W. D. Oliver, J.-S. Tsai, T. Yamamoto, and Y. Nakamura, Single microwave-photon detector using an artificial $\lambda$-type three-level system, Nat. Commun. **7**, 12303 (2016).

[15] A. Opremcak, I. V. Pechenezhskiy, C. Howington, B. G. Christensen, M. A. Beck, E. Leonard, J. Suttle, C. Wilen, K. N. Nesterov, G. J. Ribeill, T. Thorbeck, F. Schlenker, M. G. Vavilov, B. L. T. Plourde, and R. McDermott, Measurement of a superconducting qubit with a microwave photon counter, Science **361**, 1239 (2018).

[16] R. Lescanne, S. Deléglise, E. Albertinale, U. Réglade, T. Capelle, E. Ivanov, T. Jacqmin, Z. Leghtas, and E. Flurin, Irreversible qubit-photon coupling for the detection of itinerant microwave photons, Phys. Rev. X **10**, 021038 (2020).

[17] S. Kono, K. Koshino, Y. Tabuchi, A. Noguchi, and Y. Nakamura, Quantum non-demolition detection of an itinerant microwave photon, Nat. Phys. **14**, 546 (2018).

[18] J.-C. Besse, S. Gasparinetti, M. C. Collodo, T. Walter, P. Kurpiers, M. Pechal, C. Eichler, and A. Wallraff, Single-shot quantum nondemolition detection of individual itinerant microwave photons, Phys. Rev. X **8**, 021003 (2018).

[19] Z. Wang, Z. Bao, Y. Li, Y. Wu, W. Cai, W. Wang, X. Han, J. Wang, Y. Song, L. Sun, H. Zhang, and L. Duan, An ultra-high gain single-photon transistor in the microwave regime, Nat. Commun. **13**, 6104 (2022).

[20] R. Dassonneville, R. Assouly, T. Peronnin, P. Rouchon, and B. Huard, Number-resolved photocounter for propagating microwave mode, Phys. Rev. Appl. **14**, 044022 (2020).

[21] J.-C. Besse, S. Gasparinetti, M. C. Collodo, T. Walter, A. Remm, J. Krause, C. Eichler, and A. Wallraff, Parity detection of propagating microwave fields, Phys. Rev. X **10**, 011046 (2020).

[22] J. Wei, D. Olaya, B. S. Karasik, S. V. Pereverzev, A. V. Sergeev, and M. E. Gershenson, Ultrasensitive hot-electron nanobolometers for terahertz astrophysics, Nat. Nanotechnol. **3**, 496 (2008).

[23] J. Govenius, R. E. Lake, K. Y. Tan, V. Pietilä, J. K. Julin, I. J. Maasilta, P. Virtanen, and M. Möttönen, Microwave nanobolometer based on proximity josephson junctions, Phys. Rev. B **90**, 064505 (2014).

[24] B. Karimi, F. Brange, P. Samuelsson, and J. P. Pekola, Reaching the ultimate energy resolution of a quantum detector,

Nat. Commun. **11**, 367 (2020).
[25] G.-H. Lee, D. K. Efetov, W. Jung, L. Ranzani, E. D. Walsh, T. A. Ohki, T. Taniguchi, K. Watanabe, P. Kim, D. Englund, and K. C. Fong, Graphene-based josephson junction microwave bolometer, Nature **586**, 42 (2020).
[26] J. Govenius, R. E. Lake, K. Y. Tan, and M. Möttönen, Detection of zeptojoule microwave pulses using electrothermal feedback in proximity-induced josephson junctions, Phys. Rev. Lett. **117**, 030802 (2016).
[27] R. Kokkoniemi, J. Govenius, V. Vesterinen, R. E. Lake, A. M. Gunyhó, K. Y. Tan, S. Simbierowicz, L. Grönberg, J. Lehtinen, M. Prunnila, J. Hassel, A. Lamminen, O.-P. Saira, and M. Möttönen, Nanobolometer with ultralow noise equivalent power, Commun. Phys. **2**, 124 (2019).
[28] R. Kokkoniemi, J.-P. Girard, D. Hazra, A. Laitinen, J. Govenius, R. E. Lake, I. Sallinen, V. Vesterinen, M. Partanen, J. Y. Tan, K. W. Chan, K. Y. Tan, P. Hakonen, and M. Möttönen, Bolometer operating at the threshold for circuit quantum electrodynamics, Nature **586**, 47 (2020).
[29] A. M. Gunyhó, S. Kundu, J. Ma, W. Liu, S. Niemelä, G. Catto, V. Vadimov, V. Vesterinen, P. Singh, Q. Chen, and M. Möttönen, Single-shot readout of a superconducting qubit using a thermal detector, Nat. Electron. **7**, 288 (2024).
[30] A. Keränen, Q.-M. Chen, A. Gunyhó, P. Singh, J. Ma, V. Vesterinen, J. Govenius, and M. Möttönen, Correlation measurement of propagating microwave photons at millikelvin, Nat. Commun. **16**, 3875 (2025).
[31] A. I. Lvovsky and M. G. Raymer, Continuous-variable optical quantum-state tomography, Rev. Mod. Phys. **81**, 299 (2009).
[32] F. Mallet, M. A. Castellanos-Beltran, H. S. Ku, S. Glancy, E. Knill, K. D. Irwin, G. C. Hilton, L. R. Vale, and K. W. Lehnert, Quantum state tomography of an itinerant squeezed microwave field, Phys. Rev. Lett. **106**, 220502 (2011).
[33] G. L. Zeng, *Medical Image Reconstruction: From Analytical and Iterative Methods to Machine Learning*, 2nd ed. (De Gruyter, 2023).
[34] K. J. Blow, R. Loudon, S. J. D. Phoenix, and T. J. Shepherd, Continuum fields in quantum optics, Phys. Rev. A **42**, 4102 (1990).
[35] M. Mariantoni, E. P. Menzel, F. Deppe, M. A. Araque Caballero, A. Baust, T. Niemczyk, E. Hoffmann, E. Solano, A. Marx, and R. Gross, Planck spectroscopy and quantum noise of microwave beam splitters, Phys. Rev. Lett. **105**, 133601 (2010).
[36] M. Perelshtein, K. Petrovnin, V. Vesterinen, S. Hamedani Raja, I. Lilja, M. Will, A. Savin, S. Simbierowicz, R. Jabdaraghi, J. Lehtinen, L. Grönberg, J. Hassel, M. Prunnila, J. Govenius, G. Paraoanu, and P. Hakonen, Broadband continuous-variable entanglement generation using a kerr-free josephson metamaterial, Phys. Rev. Appl. **18**, 024063 (2022).
[37] M. Esposito, A. Ranadive, L. Planat, S. Leger, D. Fraudet, V. Jouanny, O. Buisson, W. Guichard, C. Naud, J. Aumentado, F. Lecocq, and N. Roch, Observation of two-mode squeezing in a traveling wave parametric amplifier, Phys. Rev. Lett. **128**, 153603 (2022).
[38] J. Y. Qiu, A. Grimsmo, K. Peng, B. Kannan, B. Lienhard, Y. Sung, P. Krantz, V. Bolkhovsky, G. Calusine, D. Kim, A. Melville, B. M. Niedzielski, J. Yoder, M. E. Schwartz, T. P. Orlando, I. Siddiqi, S. Gustavsson, K. P. O'Brien, and W. D. Oliver, Broadband squeezed microwaves and amplification with a josephson travelling-wave parametric amplifier, Nat. Phys. **19**, 706 (2023).
[39] Q.-M. Chen, P. Singh, R. Duda, G. Catto, A. Keränen, A. Alizadeh, T. Mörstedt, A. Sah, A. Gunyhó, W. Liu, and M. Möttönen, Compact inductor-capacitor resonators at sub-gigahertz frequencies, Phys. Rev. Res. **5**, 043126 (2023).
[40] D. Donoho, Compressed sensing, IEEE Trans. Inf. Theory **52**, 1289 (2006).
[41] E. J. Candes and T. Tao, Near-optimal signal recovery from random projections: Universal encoding strategies?, IEEE Trans. Inf. Theory **52**, 5406 (2006).
[42] P. Singh, A. Gunyhó, H. Suominen, G. Catto, F. Blanchet, Q.-M. Chen, A. Alizadeh, A. Keränen, J. Ma, T. Mörstedt, W. Liu, and M. Möttönen, Multiplexed readout of ultrasensitive bolometers, arXiv:2411.12782 10.48550/arXiv.2411.12782 (2024).
[43] R. Cheng, Y. Zhou, S. Wang, M. Shen, T. Taher, and H. X. Tang, A 100-pixel photon-number-resolving detector unveiling photon statistics, Nat. Photon. **17**, 112 (2022).
[44] M. Forsch, R. Stockill, A. Wallucks, I. Marinković, C. Gärtner, R. A. Norte, F. van Otten, A. Fiore, K. Srinivasan, and S. Gröblacher, Microwave-to-optics conversion using a mechanical oscillator in its quantum ground state, Nat. Phys. **16**, 69 (2019).
[45] A. Gunyhó, K. Kohvakka, Q.-M. Chen, J.-P. Girard, R. Kokkoniemi, W. Liu, and M. Möttönen, Zeptojoule calorimetry, arXiv:2412.14079 10.48550/arXiv.2412.14079 (2024).
[46] M. A. Castellanos-Beltran, K. D. Irwin, G. C. Hilton, L. R. Vale, and K. W. Lehnert, Amplification and squeezing of quantum noise with a tunable josephson metamaterial, Nat. Phys. **4**, 929 (2008).
[47] A. Vaartjes, A. Kringhøj, W. Vine, T. Day, A. Morello, and J. J. Pla, Strong microwave squeezing above 1 tesla and 1 kelvin, Nat. Commun. **15**, 4229 (2024).
[48] N. Bergeal, F. Schackert, M. Metcalfe, R. Vijay, V. E. Manucharyan, L. Frunzio, D. E. Prober, R. J. Schoelkopf, S. M. Girvin, and M. H. Devoret, Phase-preserving amplification near the quantum limit with a josephson ring modulator, Nature **465**, 64 (2010).
[49] N. Roch, E. Flurin, F. Nguyen, P. Morfin, P. Campagne-Ibarcq, M. H. Devoret, and B. Huard, Widely tunable, nondegenerate three-wave mixing microwave device operating near the quantum limit, Phys. Rev. Lett. **108**, 147701 (2012).
[50] E. Flurin, N. Roch, F. Mallet, M. H. Devoret, and B. Huard, Generating entangled microwave radiation over two transmission lines, Phys. Rev. Lett. **109**, 183901 (2012).
